# Supplementary material for: A Beam-Space Active Sensing Scheme for Integrated Communication and Sensing Applications
Source: arXiv:2210.04312 source file (2022-10-09)
Supplement: Supplementary file 1 [file BFAppendix.tex]

\subsection{Design Specific Beam Patterns}\label{app_1}
The beam pattern design method discussed in section \ref{sec:bf_design}

%\begin{figure}
%\centering
%\scalebox{.45}{\input{track_mode_opt}}
%\caption{BS transmit beam patterns for ULA$_{128}$ and FoV$=30^{\circ}$. }
%\label{fig:trck_30_opt}
%\end{figure}

\begin{figure}[ht]
\begin{minipage}[b]{0.45\linewidth}
\centering
\scalebox{0.5}{\input{track_mode_opt}}
\caption{Optimized beams}
\label{fig:figure1}
\end{minipage}
\hspace{0.4cm}
\begin{minipage}[b]{0.45\linewidth}
\centering
\scalebox{0.5}{\input{track_mode_fr}}
\caption{Fourier beams}
\label{fig:figure2}
\end{minipage}
\end{figure}

\begin{figure}
\centering
\scalebox{.6}{\input{scan_mode_opt}}
\vspace{-1cm}
\caption{BS transmit beam patterns for ULA$_{128}$ and FoV$=30^{\circ}$,FoV$=20^{\circ}$ and FoV$=10^{\circ}$ in initial scanning mode. Note that the \textit{flat-top} beam patterns have been optimized to cover the desired FoV in uniform fashion.}
\label{fig:scan_30_opt}
\end{figure}
